# Supplementary material for: Edge State Wave Functions from Momentum-Conserving Tunneling Spectroscopy
Source: arXiv:2002.05301 ancillary file (2020-02-13)
Supplement: Supplementary file 1 [file SOM.pdf]

Supplementary Information

# Edge State Wave Functions from Momentum-Conserving Tunneling Spectroscopy


T. Patlatiuk,[1,*] C.P. Scheller,[1,*] D. Hill,[2] Y. Tserkovnyak,[2] J. C. Egues,[3] G. Barak,[4] A. Yacoby,[4] L. N. Pfeiffer,[5] K. W. West,[5] and D. M. Zumbühl[1,†]

[1] *Departement Physik, University of Basel, Klingelbergstrasse 82, CH-4056 Basel, Switzerland*

[2] *Department of Physics and Astronomy, University of California, Los Angeles, California 90095, USA*

[3] *Instituto de Física de São Carlos, Universidade de São Paulo, 13560-970 São Carlos, São Paulo, Brazil*

[4] *Department of Physics, Harvard University, Cambridge, Massachusetts 02138, USA*

[5] *Department of Electrical Engineering, Princeton University, Princeton, New Jersey 08544, USA*

[*] equally contributing authors
[†] dominik.zumbuhl@unibas.ch

**CONTENTS**

I. Sample misalignment correction 1

II. Tunneling between numerous hybrid states and lower wire modes 2

A. Tunneling from $H_0$ 2

B. Tunneling into $LW_1$ 4

C. Tunneling into $LW_2$ 6

D. Tunneling into $LW_3$ 7

E. Tunneling into $LW_4$ 8

F. Tunneling into $LW_5$ 9

III. Interpretation of the tunneling signal 10

IV. Hybridization 12

## I. SAMPLE MISALIGNMENT CORRECTION

A small misalignment of the sample coordinate system from the axis of the vector magnet was corrected using a rotation matrix. A rotation around the $x$-axis shown in Fig. S1(a) by an angle $\alpha = -3.5°$ explains the measured Hall voltages (recorded with deenergized gates) induced by magnets pointing along $Y'$ and $Z'$ directions. Such a rotation around only one axis by a rather small angle is the simplest alignment correction consistent with the measured out-of-plane components. The conductance value g($B_Y$, $B_Z$) in the sample coordinate system, see panel Fig. S1(c), was obtained using linear interpolation among the four nearest measurement points from Fig. S1(b) with coordinates ($B_{Y'}$, $B_{Z'}$) given by:

$$\begin{pmatrix} B_{Y'} \\ B_{Z'} \end{pmatrix} = \begin{pmatrix} cos(\alpha) & sin(\alpha) \\ -sin(\alpha) & cos(\alpha) \end{pmatrix} \begin{pmatrix} B_Y \\ B_Z \end{pmatrix}$$

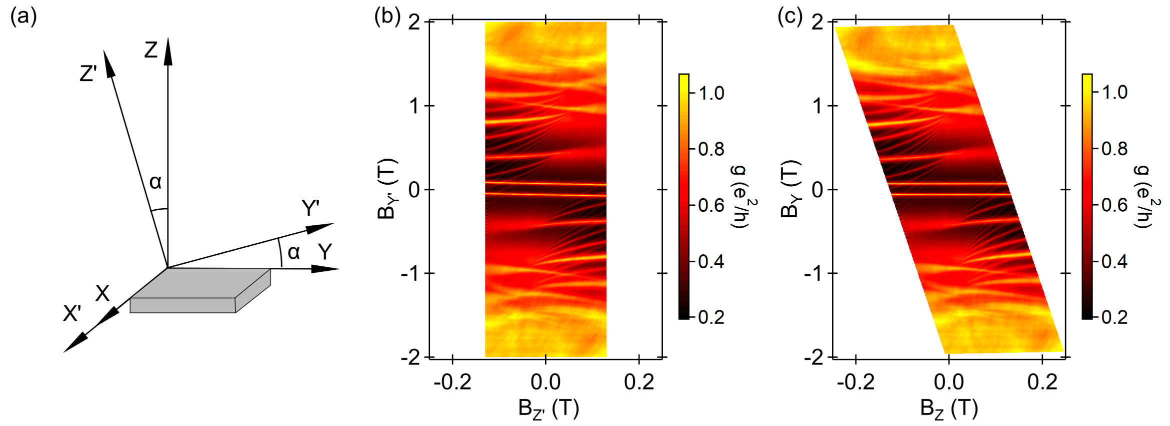


FIG. S1. (a) The magnet axis (X'Y'Z') and the sample axis (XYZ). (b) Conductance measurements in the original basis (magnet axis). (c) Conductance measurements after correcting for the sample misalignment.

## II. TUNNELING BETWEEN NUMEROUS HYBRID STATES AND LOWER WIRE MODES

The regions of substantial spatial overlap between hybrid state and lower wire wave functions are highlighted with dashed rectangles in Fig. S2,Fig. S3,Fig. S5–Fig. S8. The top and bottom boundaries of these rectangles are defined as the lines for which the normalized wave functions drop below a small predefined value, here $5 \times 10^{-4}$. The left and right boundaries are defined in a similar way by the more narrow wave function of the two in the $y$-direction. The pair of wave functions with the strongest overlap for a given magnetic field $B_Z$ (row) is highlighted with a dashed green rectangle in Fig. S3,Fig. S5–Fig. S8.

### A. Tunneling from $H_0$

The wave function of the hybrid state $H_0$ and lower wire modes $LW_2$, $LW_3$, $LW_4$, and $LW_5$ matched in $k_x$-momenta by the magnetic field $B_Y$ are shown in the first, second, third, and forth columns in Fig. S2. The magnitude of the overlap normalized to its global maximum value in Fig. 2(c) of the main text is indicated as a numeric value in each panel. Tunneling to wire modes $LW_{2,3,4,5}$ is strongly suppressed due to wave function orthogonality. In contrast, the normalized overlap between $H_0$ and the lower wire mode $LW_1$ reaches the maximal value of 1. Corresponding wave functions are shown in the first column in Fig. S3.

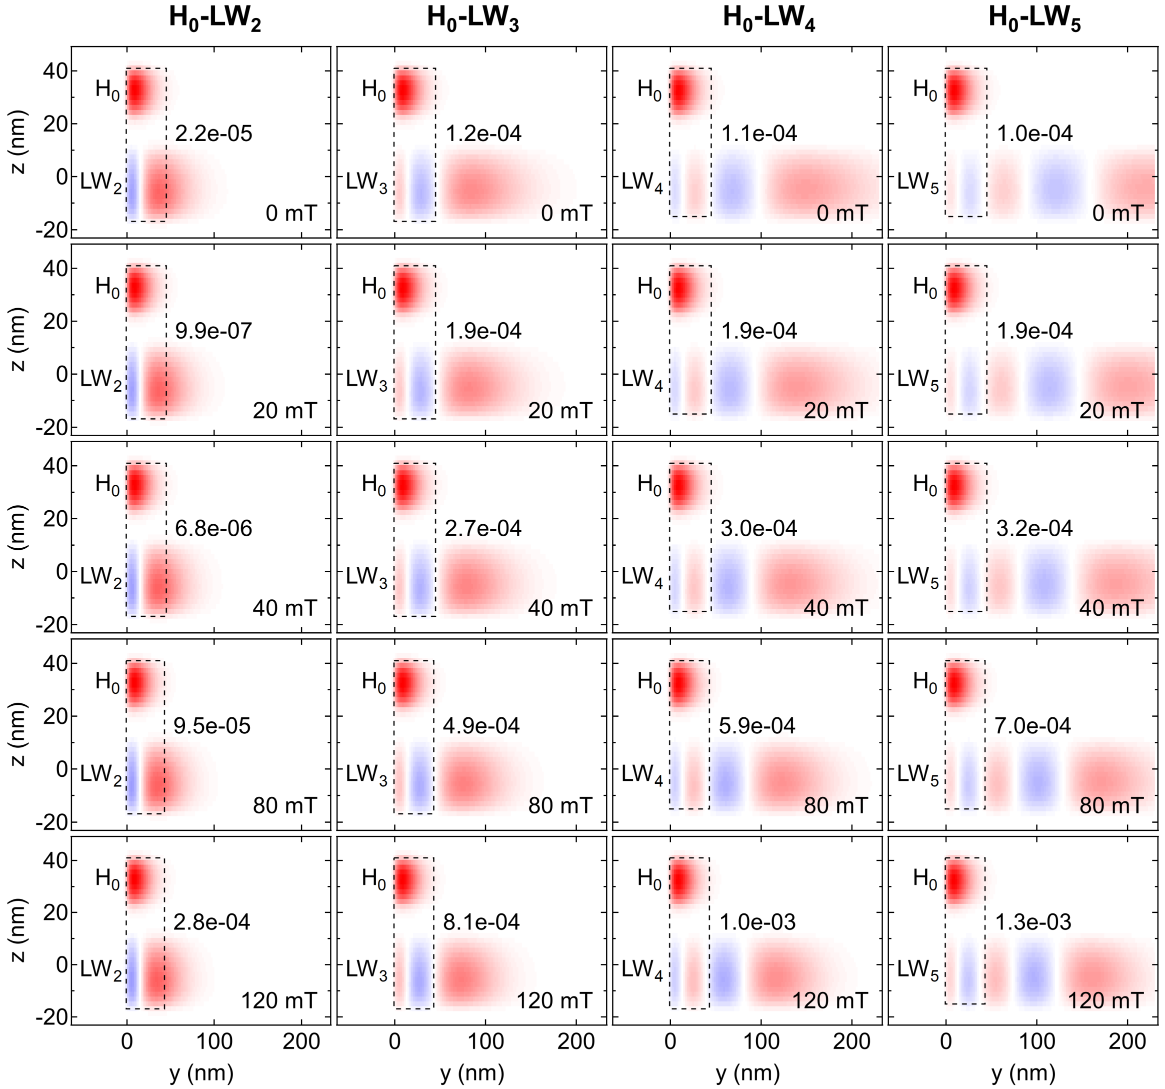


FIG. S2. The wave function of the hybrid state $H_0$ in the upper quantum well brought into resonance with the lower wire modes $LW_2$, $LW_3$, $LW_4$ and $LW_5$ calculated for a number of magnetic field values $B_Z$ as indicated. The dashed rectangle highlights the regions of substantial overlap between the wave functions. The magnitude of this overlap normalized to the global maximum overlap in Fig. 2(c) of the main text is indicated as a numeric value in each panel. None of the rectangles is highlighted in green, as all these resonances are very weak.

### B. Tunneling into $LW_1$

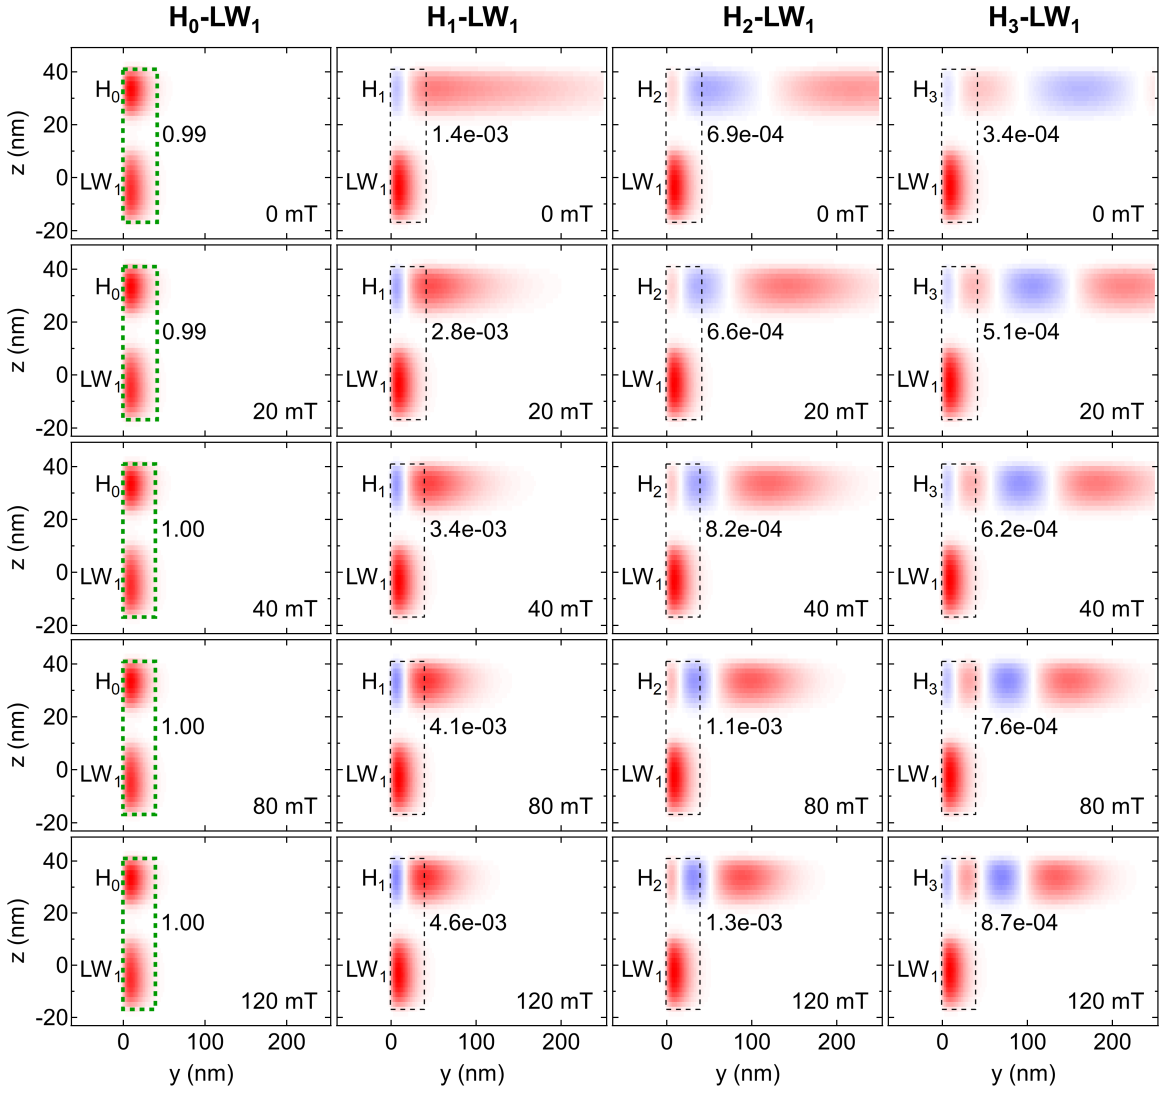


FIG. S3. The wave function of the hybrid states $H_0$, $H_1$, $H_2$, $H_3$, and wire mode $LW_1$ calculated for a number of perpendicular magnetic field values $B_Z$ as indicated. The dashed rectangle highlights the regions of substantial overlap between the wave functions. The magnitude of this overlap normalized to the global maximum overlap in Fig. 2(c) of the main text is indicated as a numeric value in each panel. The pair of wave functions with the strongest overlap for a given magnetic field $B_Z$ (row) is highlighted with a green color.

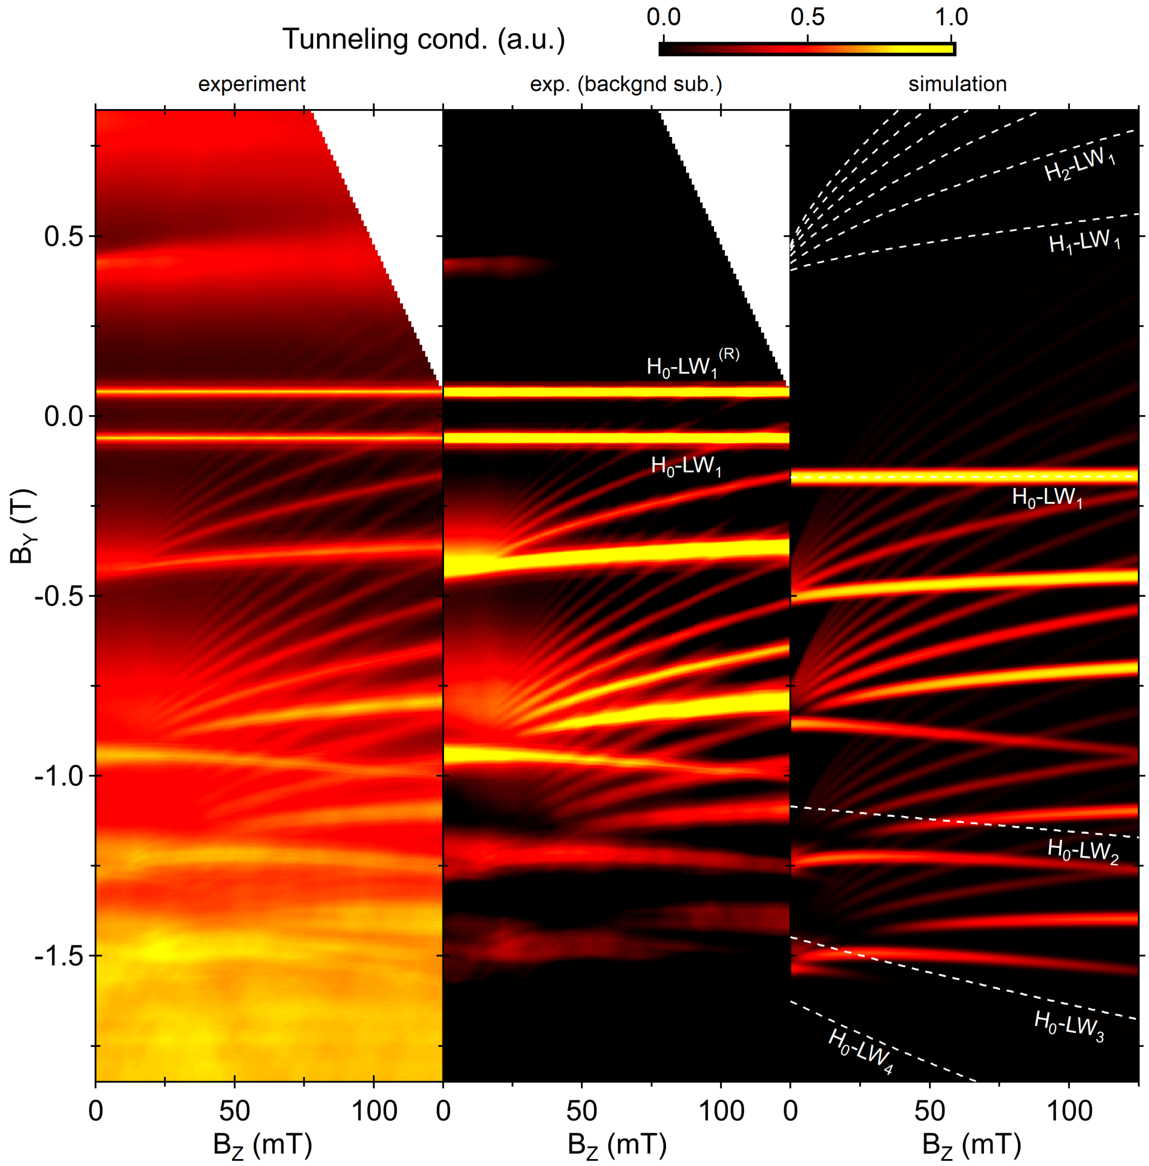


FIG. S4. The normalized tunneling conductance with (left) and without (middle) the smoothly varying background. The range of the magnetic field $B_Y$ is wider compared to Fig. 2 of the main text. The calculated tunneling conductance to the lower wire modes $LW_{1,2,3,4,5}$ is shown in the right panel. The tunneling to the lower wire mode $LW_1$ is very weak for all the hybrid states except $H_0$. The white dashed curves at the top of the right panel indicate the predicted position of the resonances $H_1 - LW_1, H_2 - LW_1, \ldots$. Three dashed curves at the bottom of the right panel indicate the predicted position of the suppressed resonances $H_0 - LW_2$, $H_0 - LW_3$, and $H_0 - LW_4$ (see Fig. S2 for details). In agreement with the simulations, all the resonances marked with the dashed curves are not observed in the measurements (left and middle panels).

## C. Tunneling into $LW_2$

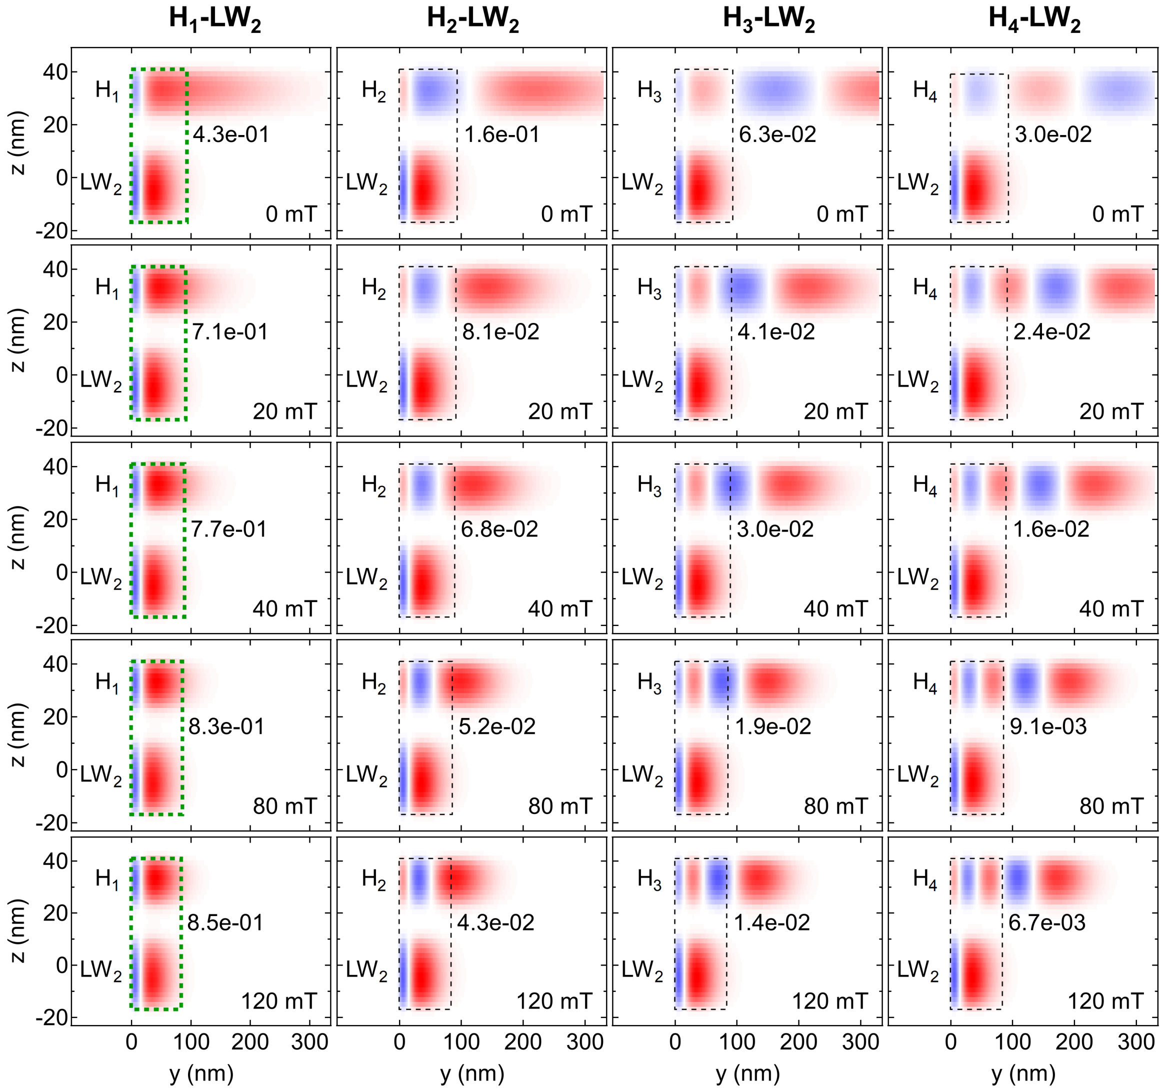


FIG. S5. The wave function of the hybrid states $H_1, H_2, H_3$, $H_4$, and wire mode $LW_2$ calculated for a number of perpendicular magnetic field values $B_Z$ as indicated. The dashed rectangle highlights the regions of substantial overlap between the wave functions. The magnitude of this overlap normalized to the global maximum overlap in Fig. 2(c) of the main text is indicated as a numeric value in each panel. The pair of wave functions with the strongest overlap for a given magnetic field $B_Z$ (row) is highlighted with a green color.

### D. Tunneling into $LW_3$

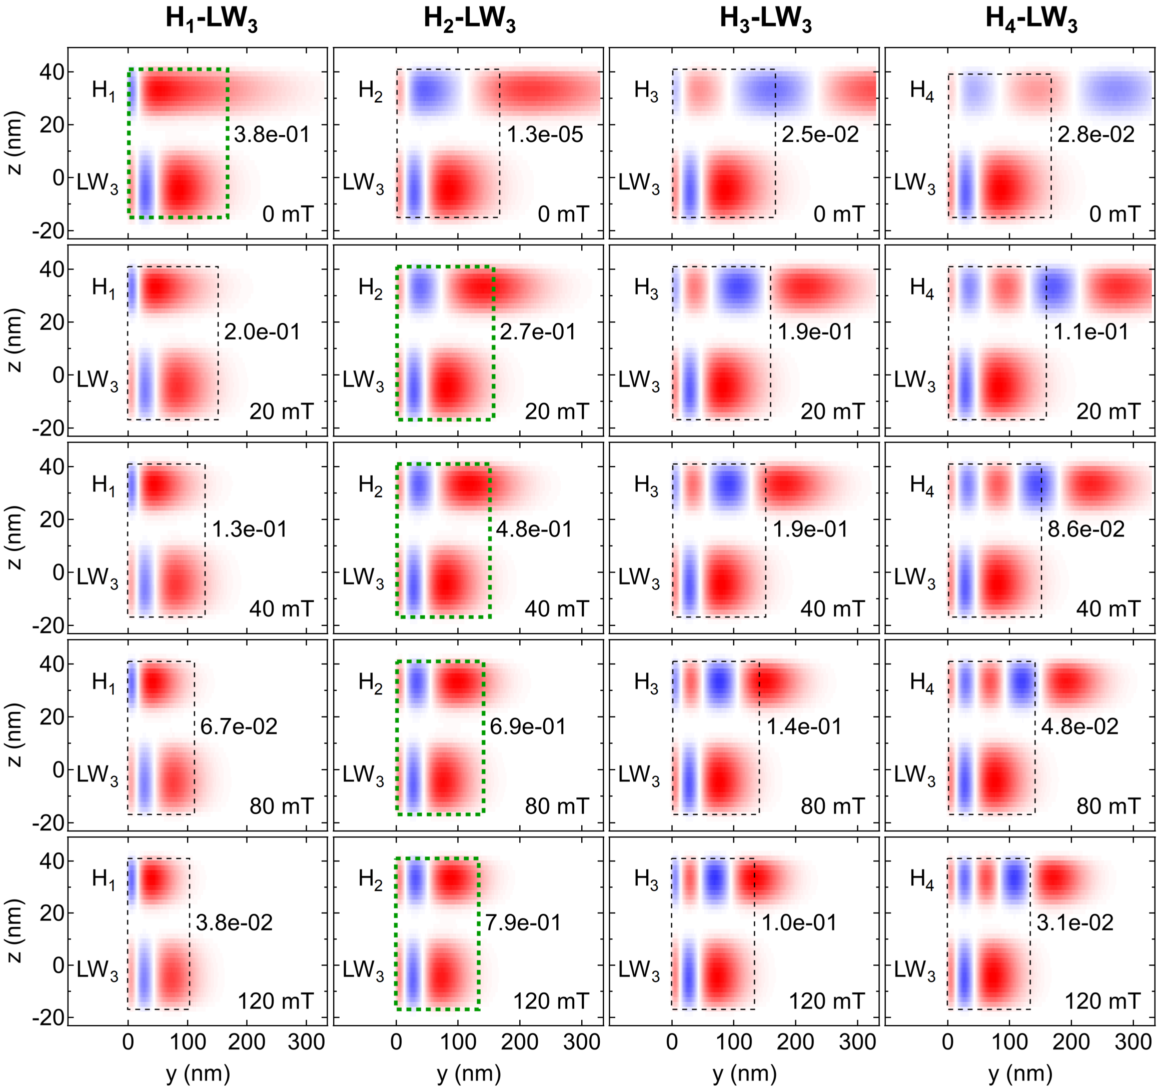


FIG. S6. The wave function of the hybrid states $H_1, H_2, H_3$, $H_4$, and wire mode $LW_3$ calculated for a number of perpendicular magnetic field values $B_Z$ as indicated. The dashed rectangle highlights the regions of substantial overlap between the wave functions. The magnitude of this overlap normalized to the global maximum overlap in Fig. 2(c) of the main text is indicated as a numeric value in each panel. The pair of wave functions with the strongest overlap for a given magnetic field $B_Z$ (row) is highlighted with a green color.

## E. Tunneling into $LW_4$

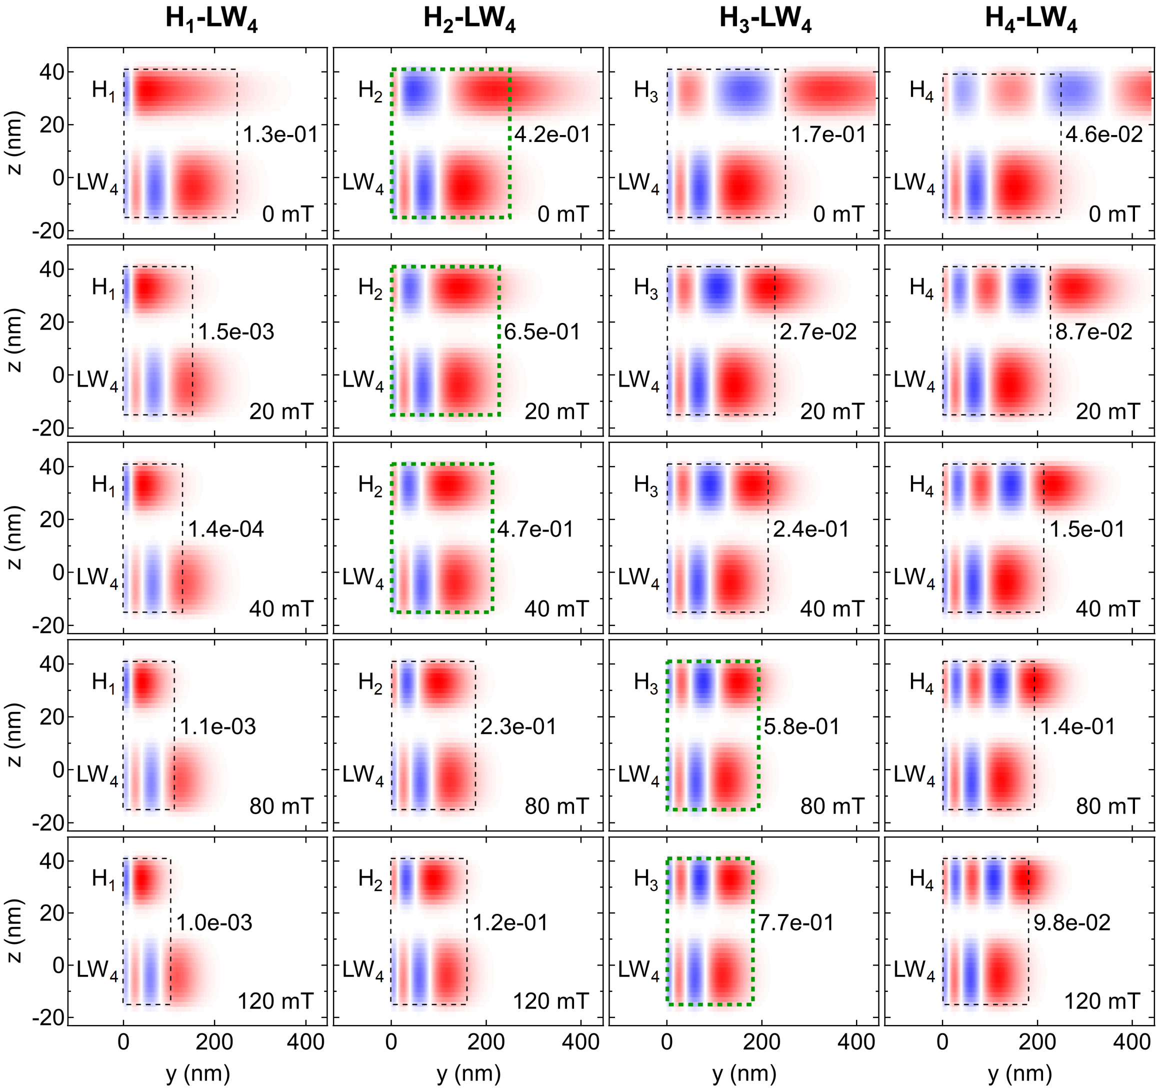


FIG. S7. The wave function of the hybrid states $H_1, H_2, H_3$, $H_4$, and wire mode $LW_4$ calculated for a number of perpendicular magnetic field values $B_Z$ as indicated. The dashed rectangle highlights the regions of substantial overlap between the wave functions. The magnitude of this overlap normalized to the global maximum overlap in Fig. 2(c) of the main text is indicated as a numeric value in each panel. The pair of wave functions with the strongest overlap for a given magnetic field $B_Z$ (row) is highlighted with a green color.

## F. Tunneling into $LW_5$

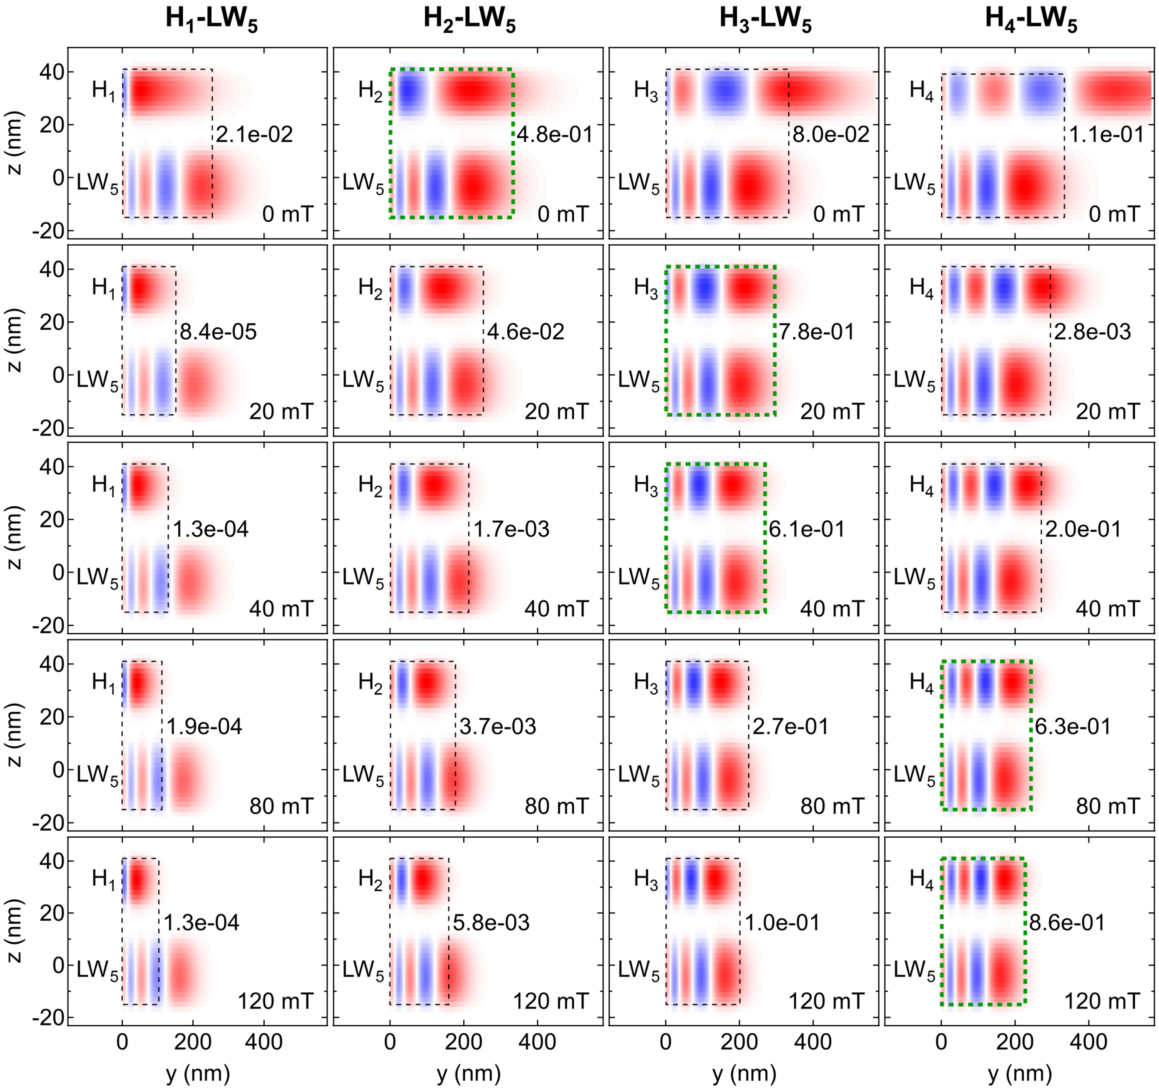


FIG. S8. The wave function of the hybrid states $H_1, H_2, H_3$, $H_4$, and wire mode $LW_5$ calculated for a number of perpendicular magnetic field values $B_Z$ as indicated. The dashed rectangle highlights the regions of substantial overlap between the wave functions. The magnitude of this overlap normalized to the global maximum overlap in Fig. 2(c) of the main text is indicated as a numeric value in each panel. The pair of wave functions with the strongest overlap for a given magnetic field $B_Z$ (row) is highlighted with a green color.

## III. INTERPRETATION OF THE TUNNELING SIGNAL

To visualize the origin of tunneling conductance variations we plot the wave function cross sections along the $y$-direction for $z = 0$ (upper system) and $z = 31\,\mathrm{nm}$ (lower system), Fig. S9(a,b), corresponding to the center of the upper and lower quantum wells, respectively. Solid curves correspond to the cross sections of the hybrid states $H_1$ (panel a) and $H_2$ (panel b), while dashed curves correspond to the cross section of the wave function of the lower wire $LW_3$. The values of the magnetic field $B_Z$ are labeled and color coded.

At zero magnetic field, the comparably soft upper system confinement potential forms a strongly asymmetric wave function of the hybrid state $H_1$ which has only one node (solid red curve). The strong and wide second lobe of this wave function protrudes deeply into the bulk of the sample. As the magnetic field $B_Z$ is increased, the width of this lobe reduces significantly. In contrast, the wave function of the lower wire mode $LW_3$ is modified only slightly by magnetic field, due to the stronger triangular confinement potential along the $y$-direction in the lower system, see Fig. 1(c) in the main text.

The exponential decay of the wave function inside the AlGaAs barrier as well as the wave function profiles in the $y$-direction determine the strength of the overlap, given by the product of the $y$-wave function profiles in upper and lower system, shown in panel (c). The products integrated along the $y$-direction are shown in panel (e). At $Bz = 0$ (red) the product of the wave function profiles has two small negative lobes and one wide positive lobe, which dominates the integrated value. As the magnetic field $B_Z$ is increased, the strength of the negative lobes is increased. At the same time, the width of the positive lobe is reduced. As a consequence, the result of the integration that is directly related to the wave function overlap is also reduced. This explains the reduction of the tunneling conductance of the $H_1 - LW_3$ resonance as the magnetic field $B_Z$ increases.

The right column of Fig. S9 shows the wave functions (b), their products (d), and result of integration for the hybrid state $H_2$ and lower wire mode $LW_3$. In this case, the small overlap at small $B_Z$ is caused by different length scale of the wave functions that becomes comparable at higher fields. As a consequence, the tunneling conductance of the $H_2 - LW_3$ resonance is very small at small $B_Z$ and rapidly increases in the presence of magnetic field along the $z$-direction.

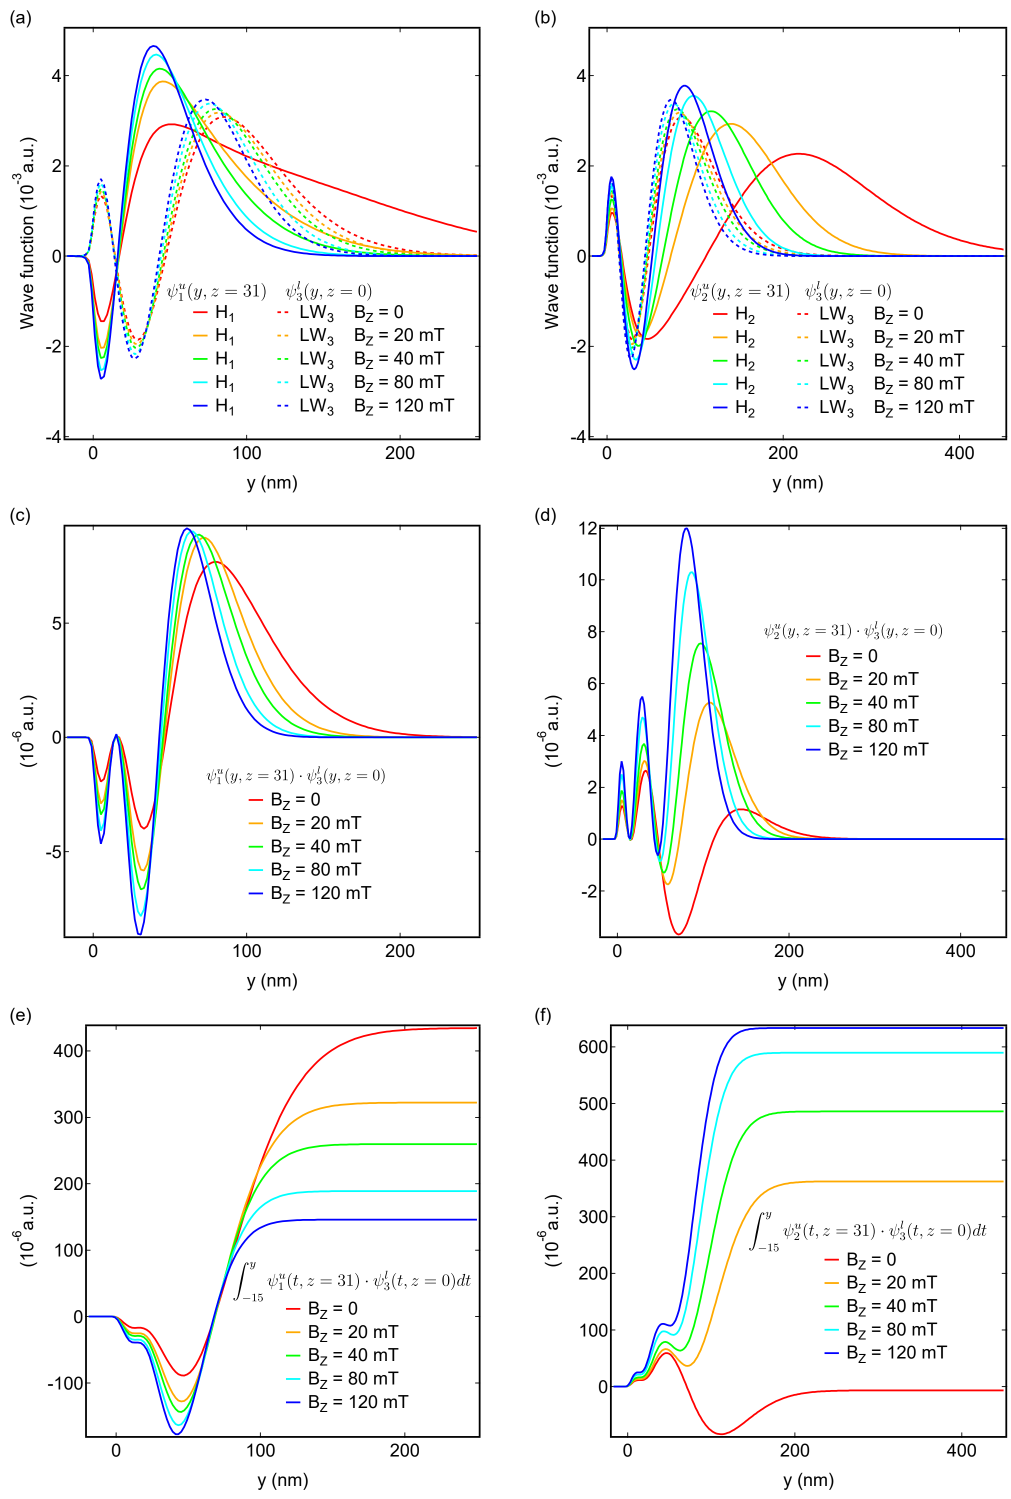


FIG. S9. (a) The cross section along the $y$-direction of the wave functions of hybrid state $H_1$ in the upper system ($z = 31$ nm) and wire mode $LW_3$ ($z = 0$) in the lower system at several magnetic fields $B_Z$. (b) Similar to (a) but for state $H_2$ in the upper system. (c,d) The product of upper system and lower system wave function cross sections from panels (a) and (b), respectively. (e,f) The result of integration of the products from panels (c) and (d). All position coordinates are given in nanometers.

## IV. HYBRIDIZATION

The background conductance during the measurement shown in Fig. 5 of the main text was suppressed by reducing the size of the source region to 22 $\mu$m using another surface gate. This gives weak parallel replicas of observed resonances, likely originating from a nonuniform density in the source region.

The tunneling conductance measured also for the negative values of magnetic field $B_Z$ is shown in Fig. S10. The direction of edge state propagation is reversed for negative $B_Z$ and the dispersion relation is mirrored on the vertical axis (see left insets). As a result, the resonance that tracks the wire-like states for one sign of $B_Z$ will track the avoided crossings for the opposite sign of $B_Z$.

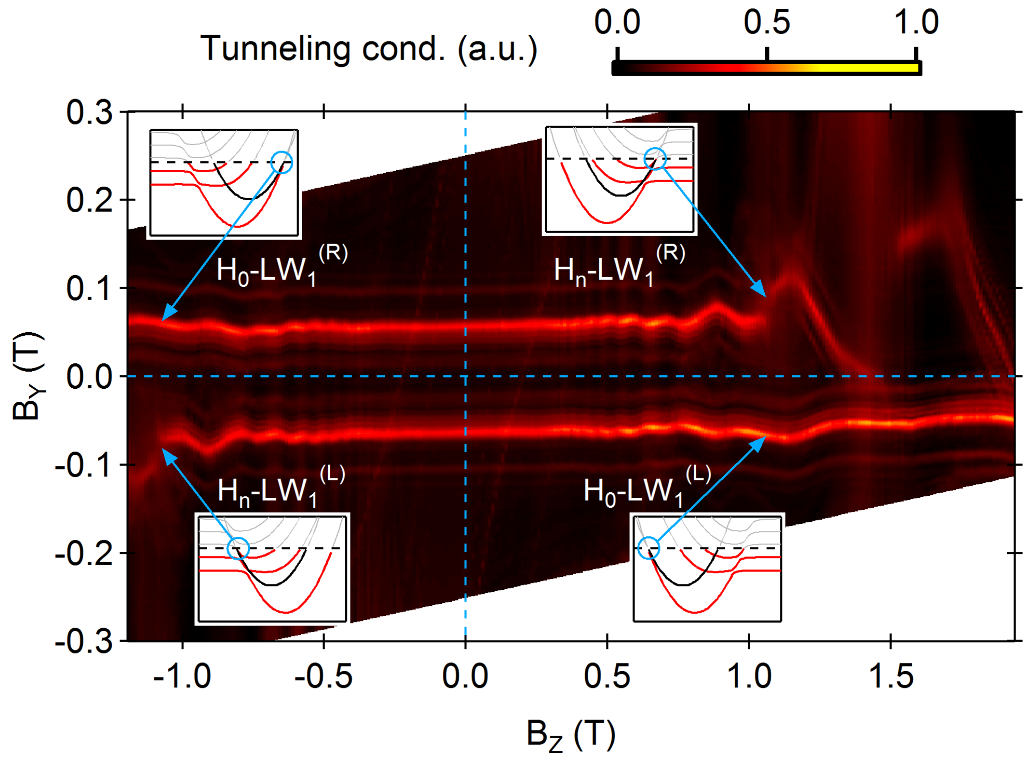


FIG. S10. Tunneling conductance between hybrid states in the upper system and the lower wire mode $LW_1$. Insets qualitatively depict the dispersion relation of the hybrid states (red) and $LW_1$ (black) for $B_Y$ and $B_Z$ which satisfy the resonant tunneling condition.
